# Supplementary material for: The Cambrian Explosion of Mixed-Precision Matrix Multiplication for Quantized Deep Learning Inference
Source: arXiv:2506.11728 source file (2025-06-13)
Supplement: Supplementary file 1 [file sn-appendix.tex]

\appendix

\begin{figure}[t!]
\begin{center}
\begin{minipage}[t]{\textwidth}
\begin{lstlisting}[language=C,alsoletter={.},deletekeywords={.sum},morekeywords={},breaklines=true]                
mv t0, %7             //Load ldC                      
mv a0, %5             //C0 Address              
add a1, a0, t0        //C1 Address             
add a2, a1, t0        //C2 Address                  
add a3, a2, t0        //C3 Address        
mv t1, %3             //Load A Address                   
mv t0, %4             //Load B Address                   
mv t3, %2             //Load KC value
vle32.v v2, (a1)      //Load 4 elements of C1                 
vle32.v v3, (a3)      //Load 4 elements of C3                  
vslideup.vi v0, v2, 4         
vslideup.vi v1, v3, 4
vle32.v v0, (a0)      //Load 4 elements of C0               
vle32.v v1, (a2)      //Load 4 elements of C2

vmadot_loop_kc:                 
  vle8.v v10, (t1)    //Load 32 elements of A        
  addi t1, t1,  32    //Update A address
  vle8.v v11, (t0)    //Load 32 elements of B                
  addi t0, t0,  32    //Update B address          
  vmadot v0, v10, v11 //Dot product                       
  addi t3, t3, -1                    
  bne  t3, zero, vmadot_loop_kc  
  
vslidedown.vi v2, v0, 4            
vslidedown.vi v3, v1, 4              
vse32.v v0, (a0)      //Store 4 elements of C0               
vse32.v v2, (a1)      //Store 4 elements of C1     
vse32.v v1, (a2)      //Store 4 elements of C2     
vse32.v v3, (a3)      //Store 4 elements of C3
\end{lstlisting}
\end{minipage}
\end{center}
\caption{vmadot IME implementation.}
\label{fig:qGEMM_microkernel_16x4_INT8_INT32_RVV}
\end{figure}
